# Supplementary material for: Lite Pose: Efficient Architecture Design for 2D Human Pose Estimation
Source: arXiv:2205.01271 source file (2022-07-11)
Supplement: Supplementary file 1 [file Appendix.tex]

\appendix

\section{Appendix}

\myparagraph{Searched Architectures}

\begin{wrapfigure}{r}{0.5\textwidth}
\vspace{-33pt}
\begin{center}
	\includegraphics[height=0.33\textwidth]{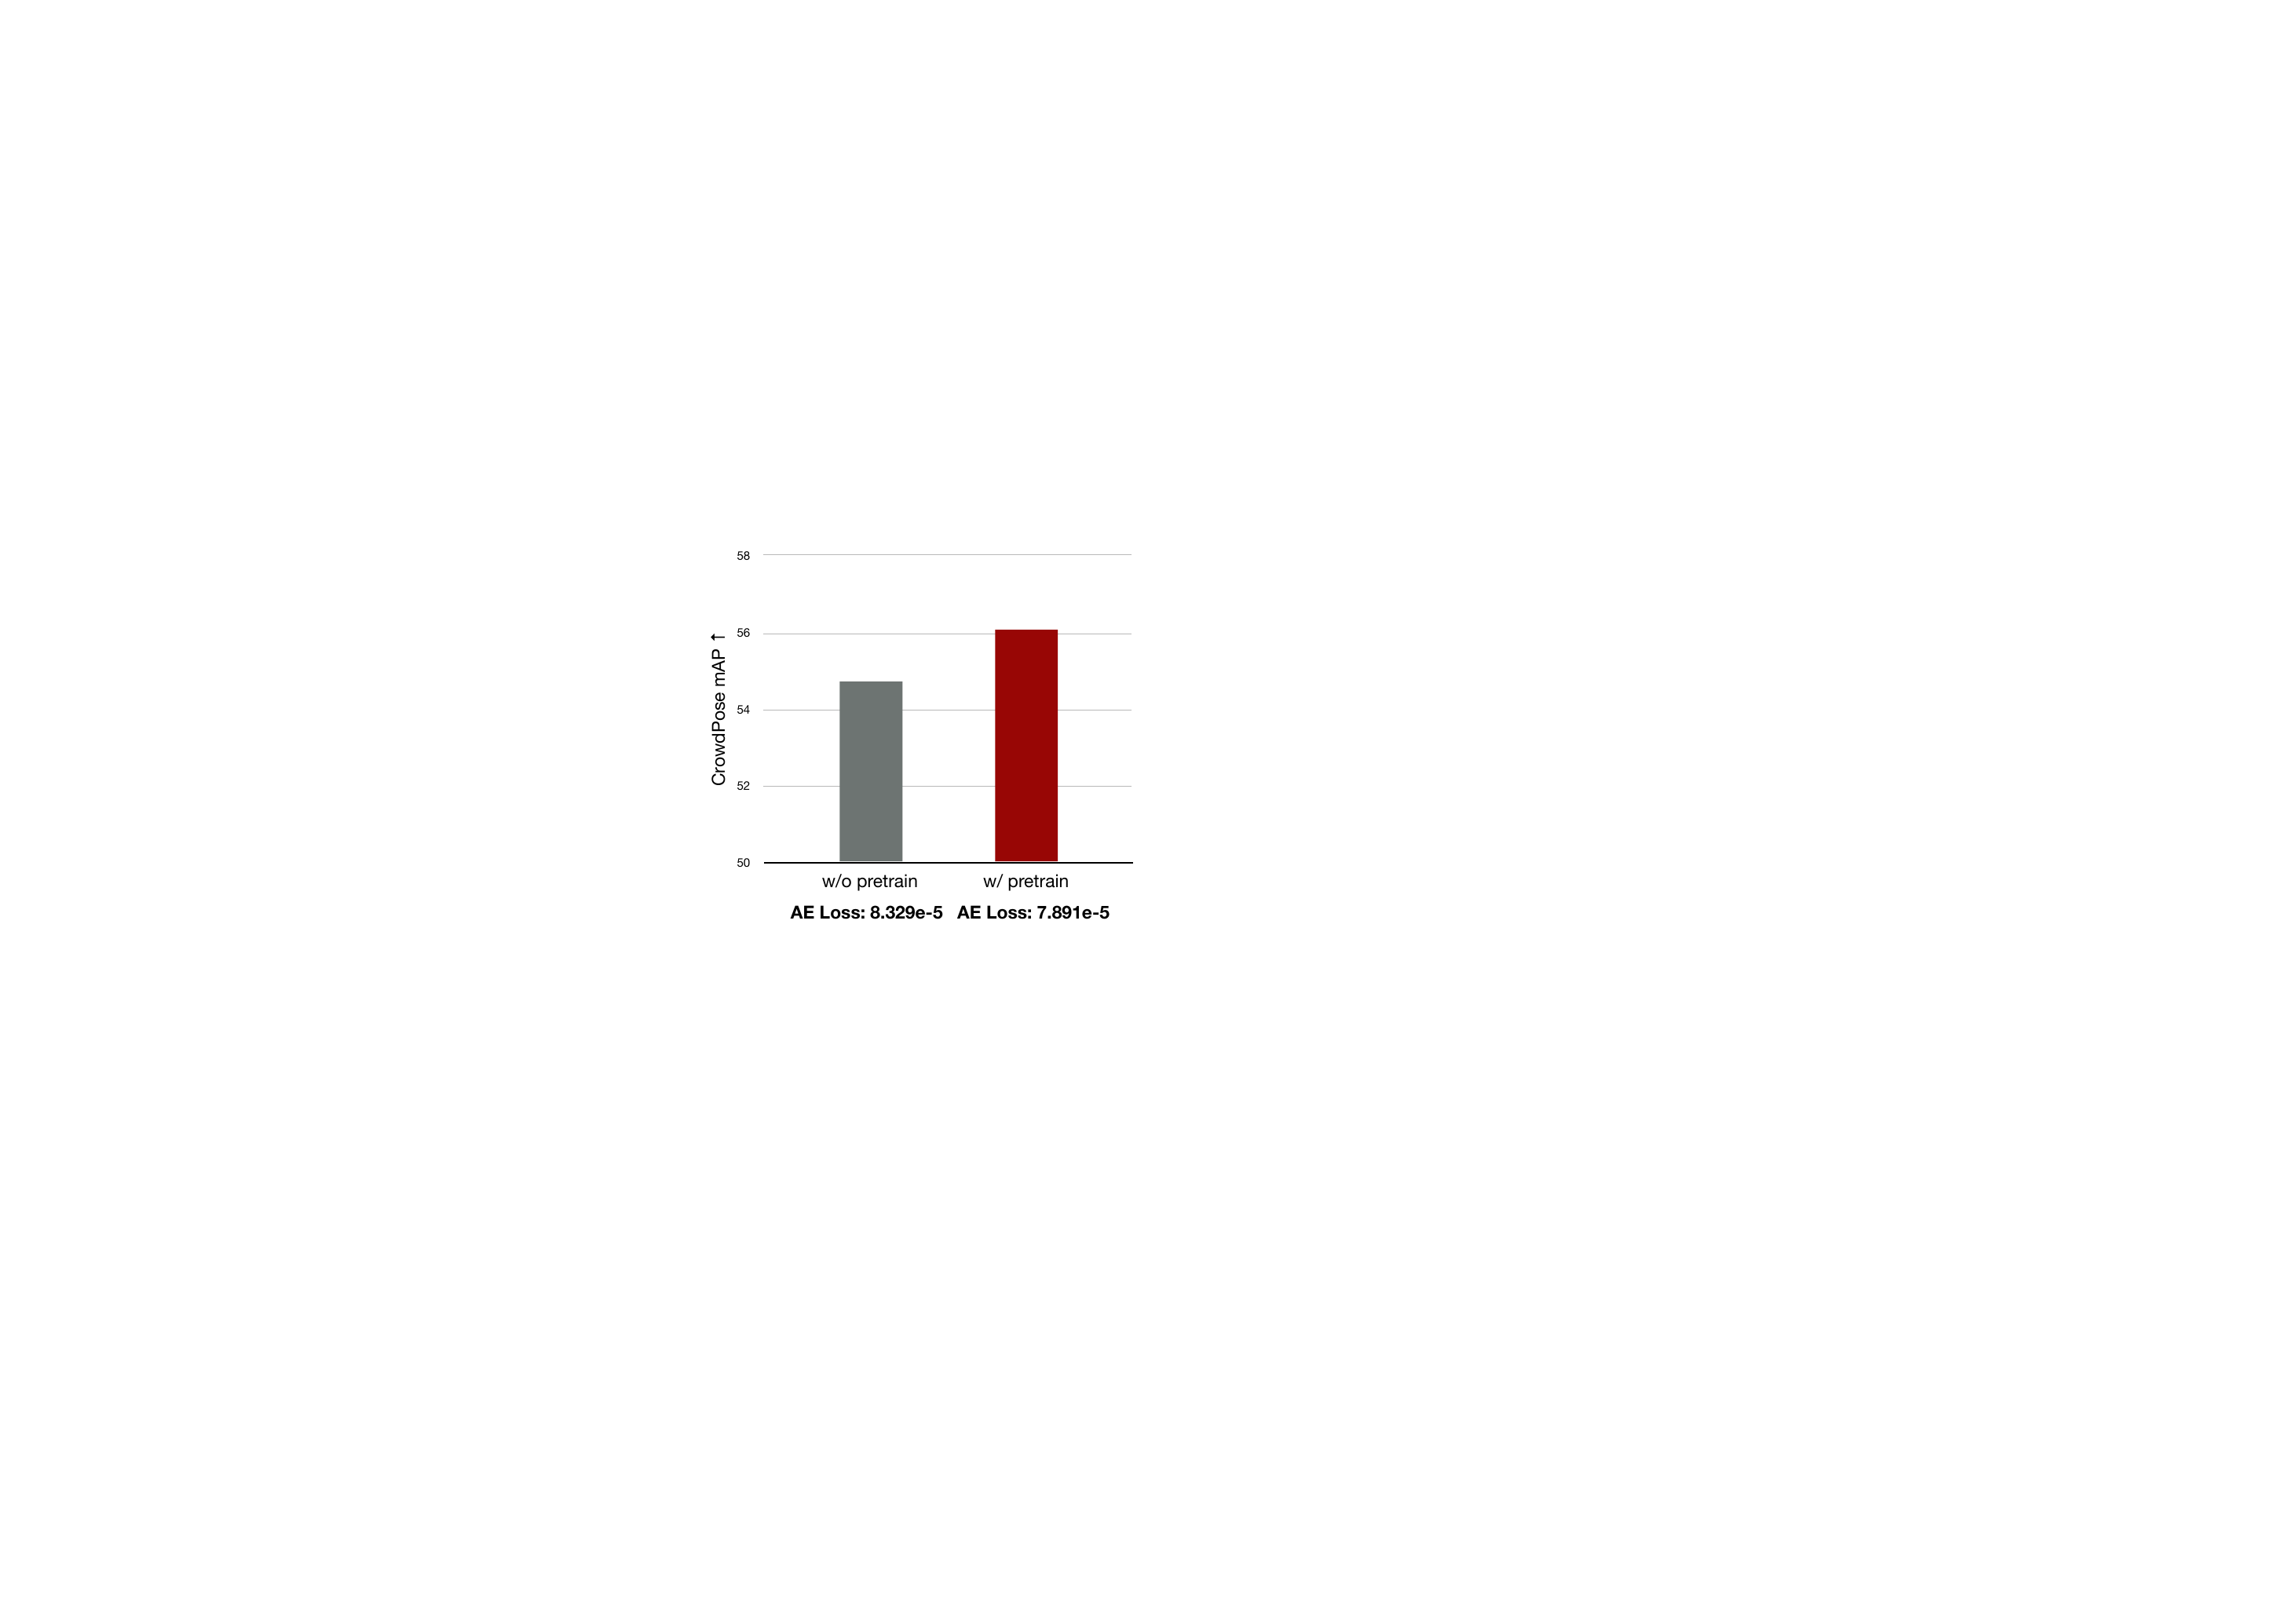}
\end{center}
\vspace{-10pt}
\caption{Pre-train ablations. With the help of pre-training trick, the model achieves higher performance and lower AE Loss.}
\label{fig:5-pretrain}
\vspace{-10pt}
\end{wrapfigure}

We put the architectures of 4 NAS architectures (\textit{LitePose-XS,S,M,L}) and their corresponding computation in Figure~\ref{fig:search-arch}. We also provide the architecture of \textit{0.5 LitePose}, which simply maintains half of the channels of the largest search space. We conduct most of our ablation experiments on \textit{0.5 LitePose}.

\myparagraph{Demos} We provide extra anonymous demos in our supplementary materials. In \textit{LitePose-S-Nano.mp4}, we present the real-time demo of \textit{LitePose-S} (optimized with AutoTVM~\cite{chen2018tvm}) on NVIDIA Jetson Nano. In \textit{Comparison.avi}, we compare the visualization performance among \textit{Lightweight OpenPose}~\cite{osokin2018real}, \textit{HigherHRNet-W24}~\cite{cheng2020higherhrnet}, and our \textit{LitePose-S} from left to right. Our \textit{LitePose-S} achieves the best visualization performance.
